# Supplementary material for: Mining User Opinions in Mobile App Reviews: A Keyword-based Approach
Source: arXiv:1505.04657 source file (2015-10-26)
Supplement: Supplementary file 1 [file appendix.tex]

\section*{Appendix}

\subsection{Skewness formula for app reviews}
	\begin{equation}
	sum = \sum_{i=1}^{5}\rho_i
	\label{eq:skewnessSum}
	\end{equation}
	\begin{itemize}
	\item $\rho_i$: count of rating $i$
	\end{itemize}	

	\begin{equation}
	\overline{\rho} = \frac{\sum_{i=1}^{5}(\rho_i \times i))}{sum}
	\label{eq:skewnessMean}
	\end{equation}
	\begin{itemize}
	\item $\overline{\rho}$: sample mean of rating counts
	\end{itemize}

	\begin{equation}
	\begin{split}
	skewness = \frac{m_3}{s_3} \times log_2(sum)\\ =\frac{\frac{1}{sum} \times \sum_{i=1}^{5}\rho_i\times (i - \overline{\rho})^{3}}{[\frac{1}{sum} \times \sum_{i=1}^{5}\rho_i \times (i - \overline{\rho})^{2}]^{\frac{3}{2}}}\times log_2(sum)
	\label{eq:skewness}
	\end{split}
	\end{equation}
	\begin{itemize}
	\item $m_3$: sample third central moment
	\item $s$: sample standard deviation
	\end{itemize}
	
\subsection{Pearson correlation formula for app reviews}

	\begin{equation}
	r = \frac{\sum XY - \frac{\sum X\sum Y}{5}}{\sqrt{\sum X^{2}-\frac{(\sum X)^{2}}{5}}\sqrt{\sum Y^{2}-\frac{(\sum Y)^{2}}{5}}}
	\label{eq:pearson}
	\end{equation}
	\begin{itemize}
	\item $X\{1,2,3,4,5\}$: the ratings
	\item $Y$: an array of rating counts, from rate 1 to rate 5
	\end{itemize}	

\subsection{Cosine Similarity}	
	\begin{equation}
	similarity = \cos(\theta) = \frac{A\cdot B}{\left \| A \right \|\left \| B \right \|}
	\label{eq:cossim}
	\end{equation}
	\begin{itemize}
	\item $A, B$: two vectors of attributes.
	\item $\cos(\theta)$: Cosine Similarity
	\end{itemize}

\subsection{Term Frequency - Document Frequency}	

	\begin{equation}
	tf.idf = \tfrac{N}{1 + log(n_{t})}
	\label{eq:tfidf}
	\end{equation}
	\begin{itemize}
	\item $N$: term frequency
	\item $n_{t}$: document frequency
	\end{itemize}

\subsection{Simple Moving Average}	
	\begin{equation}
	 \mu_i = \frac{\sum_{j=i-w}^{i-1}V_j}{w}
	\label{eq:sma}
	\end{equation}
	\begin{itemize}
	\item $\mu_i$: Simple Moving Average on day $i$
	\item $w$: Sliding window's size in days
	\item $V_j$: observed value on the timeseries on day $j$
	\end{itemize}
		
	\begin{equation}
	 \sigma = \sqrt{\frac{1}{N}\sum_{i=1}^{N}(V_i - \mu_i)^{2}}
	\label{eq:standarder}
	\end{equation}
	\begin{itemize}
	\item $\sigma$: Standard deviation of the timeseries to Simple Moving Average
	\item $N$: length of the time series in days
	\end{itemize}
